# Supplementary material for: Interpretable neural architecture search and transfer learning for understanding CRISPR/Cas9 off-target enzymatic reactions
Source: arXiv:2305.11917 ancillary file (2023-09-29)
Supplement: Supplementary file 2 [file ExtendedDataFigures.pdf]

## Table of Contents

Extended Data Figure 1-11

Extended Data Table 1-3

Extended Data Figure 1

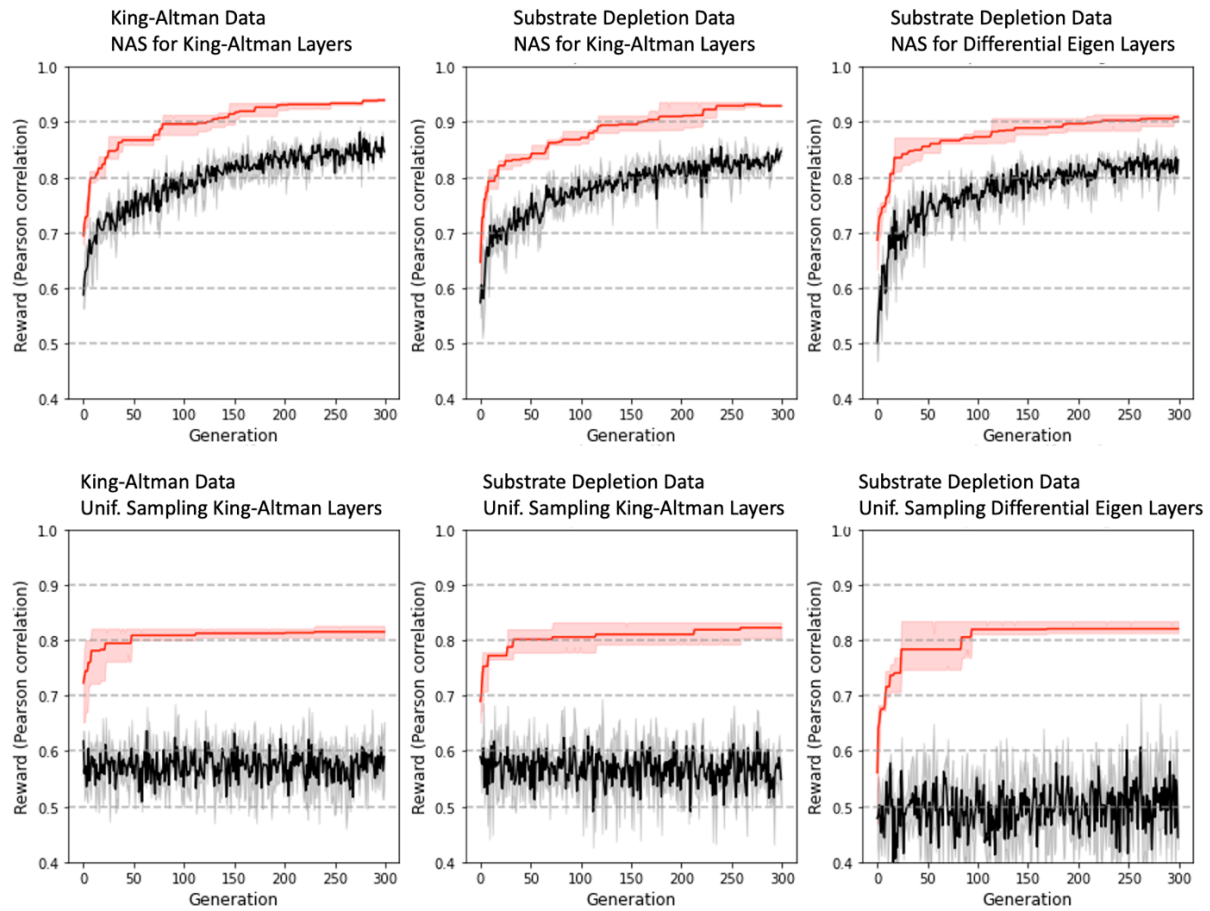

Performance of KINNs on simulated data for both steady-state data (left column) and depleting uncut DNA data (middle column). Eigen decomposition KINNs were also tested for performance against depleting uncut DNA data (right column). Top row KINN architectures were optimized through a Bayesian genetic algorithm for model building. The bottom row sampled hyperparameters uniformly during each generation. Search performance for KINNs were visualized across iterations (black lines) and for best individual model (red lines). Shaded areas are 95% confidence intervals.

Extended Data Figure 2

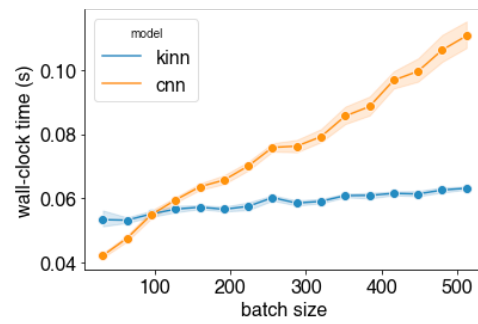

Wall-clock time comparison of training one data batch for KINN and CNN models, with varying batch sizes. Time is measured in seconds. Shaded areas are 95% confidence intervals.

Extended Data Figure 3

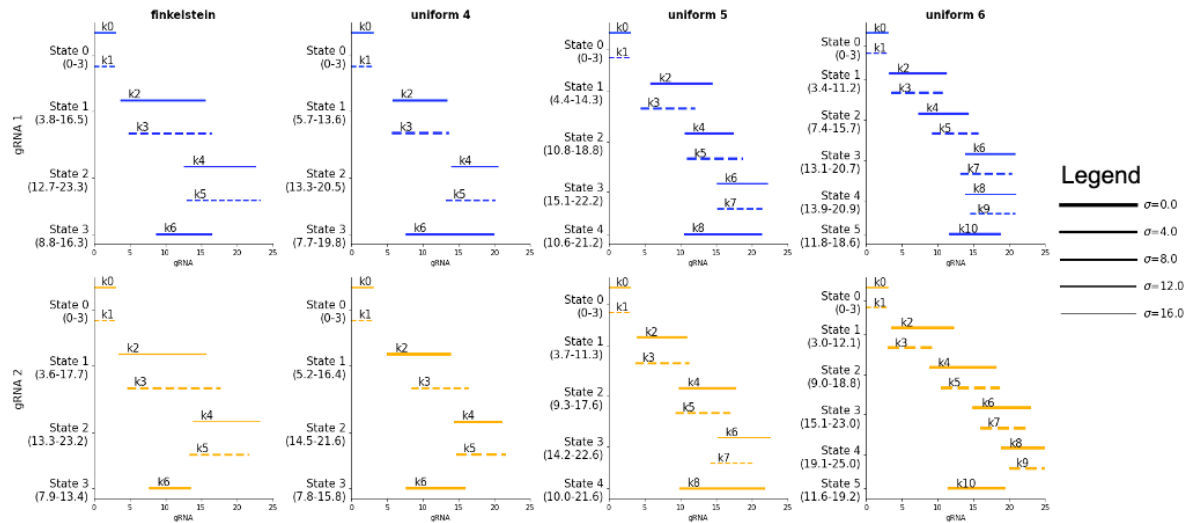

Comparison of kinetic rate sequence determinants after search and training for two different gRNA templates. Lines indicate what nucleotides contribute to the forward (solid lines) and reverse (dotted lines) reaction rate constants. Linewidth varies inversely with standard deviation between the model replicates of different KINNs with the same number of states. The zeroth state transitions, k0 and k1, were required to depend on the first 3 nucleotides corresponding to the PAM subsequence of the DNA substrate.

Extended Data Figure 4

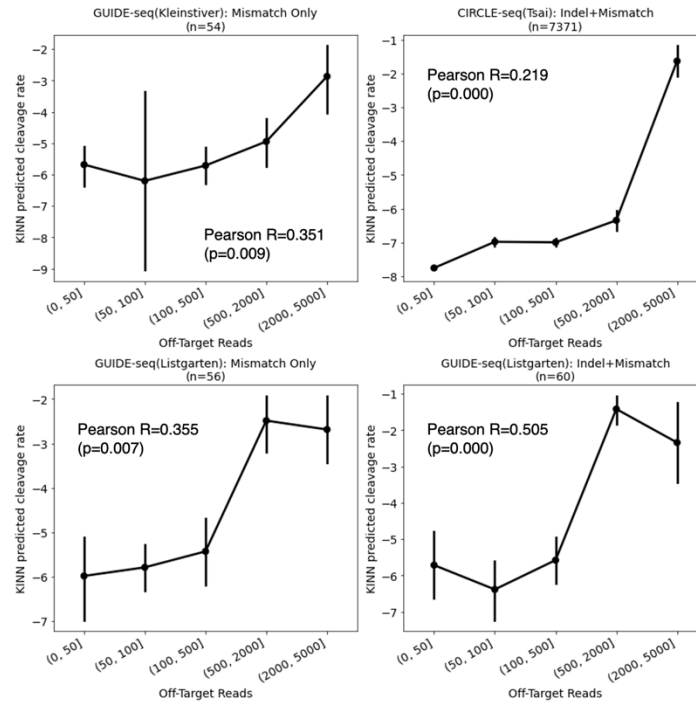

Logarithm of cleavage rates predicted by *Elektrum* as a function of *in vivo* off-target reads. Reads were binned as indicated by x-axis labels and error bars calculated by 95% confidence intervals. n is the number of detected off-target edits in each experiment.

Extended Data Figure 5

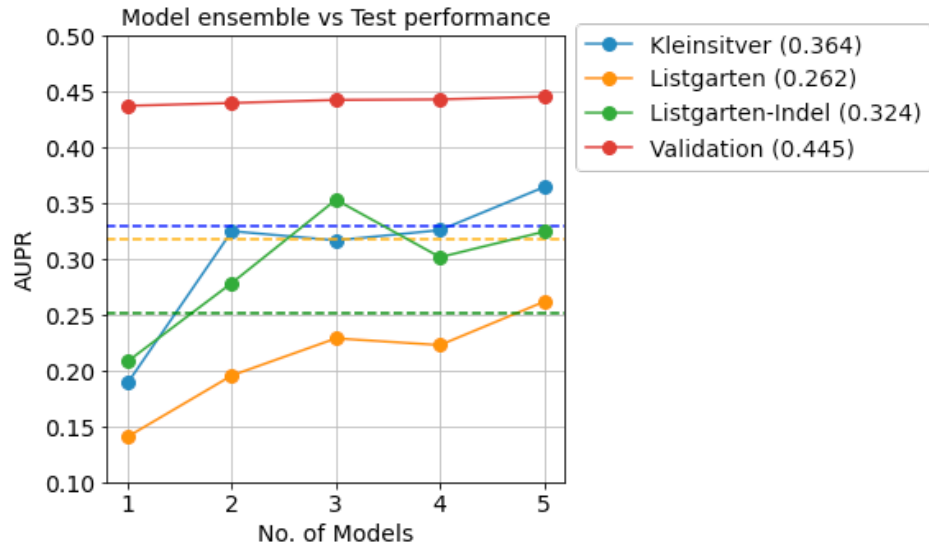

Performance of *Elektrum* as a function of the number of pre-trained KINNs in selection pool. Dotted lines are the performance of the state-of-the-art models developed in the paper corresponding to that dataset. Validation is a held-out dataset from the training data.

Extended Data Figure 6

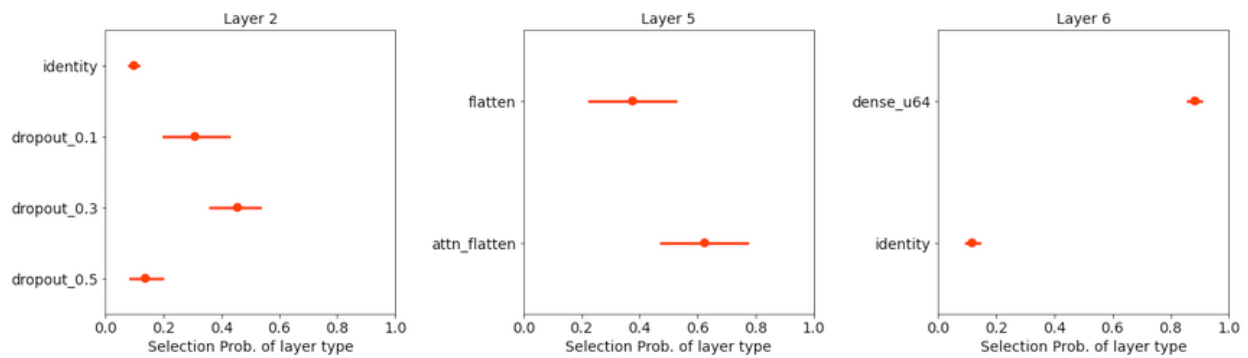

The selection probability of remaining layers for the optimal *Elektrum* model. Error bars represent the 95% confidence interval from five independent search runs.

Extended Data Figure 7

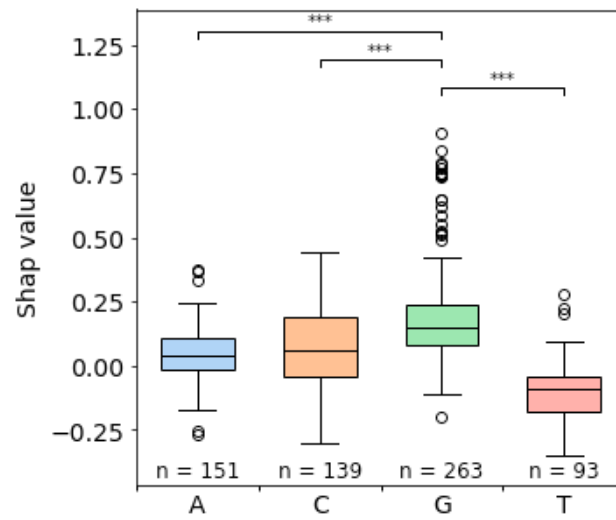

Analysis of nucleotide SHAP values in the target gRNA sequence from *Elektrum*. gRNA results were pooled from the two external test datasets.



Extended Data Figure 8

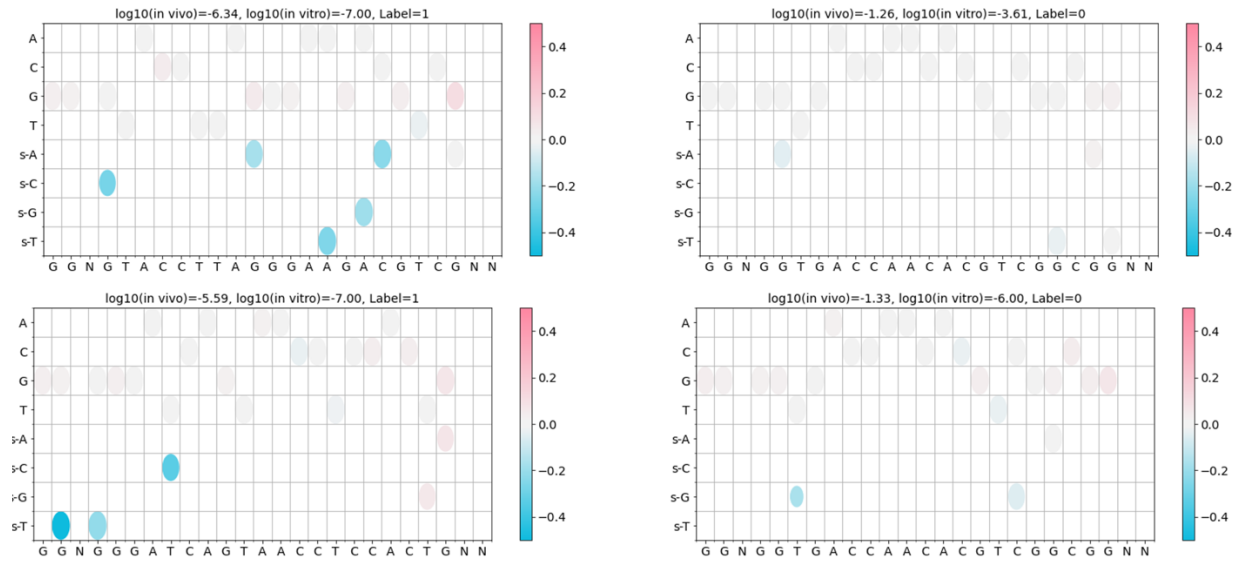

SHAP analysis for top false-positive and false-negative predictions of the *Elektrum* in-vivo model. Left row: false negatives. Right row: false positives. The gRNA sequence is shown on the x-axis. Predicted *in vivo*, *in vitro* cleavage rates and the experimental label are shown in figure titles. Color represents the average SHAP values across five best models created independently in five search runs; size of the dots scale inversely with variance of SHAP across the five models.

Extended Data Figure 9

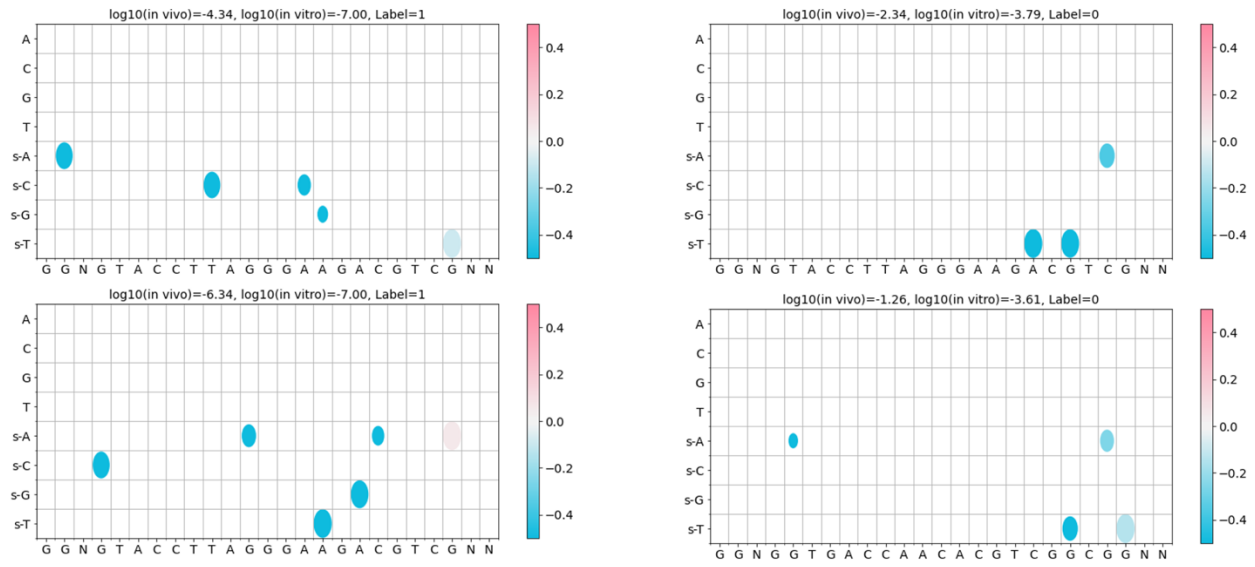

SHAP analysis for top false-positive and false-negative predictions of the *Elektrum* in-vitro models (KINNs). Left row: false negatives. Right row: false positives. The gRNA sequence is shown on the x-axis. Predicted *in vivo*, *in vitro* cleavage rates and the experimental label are shown in figure titles. Color represents the average SHAP values across five best models created independently in five search runs; size of the dots scale inversely with variance of SHAP across the five models.

Extended Data Figure 10

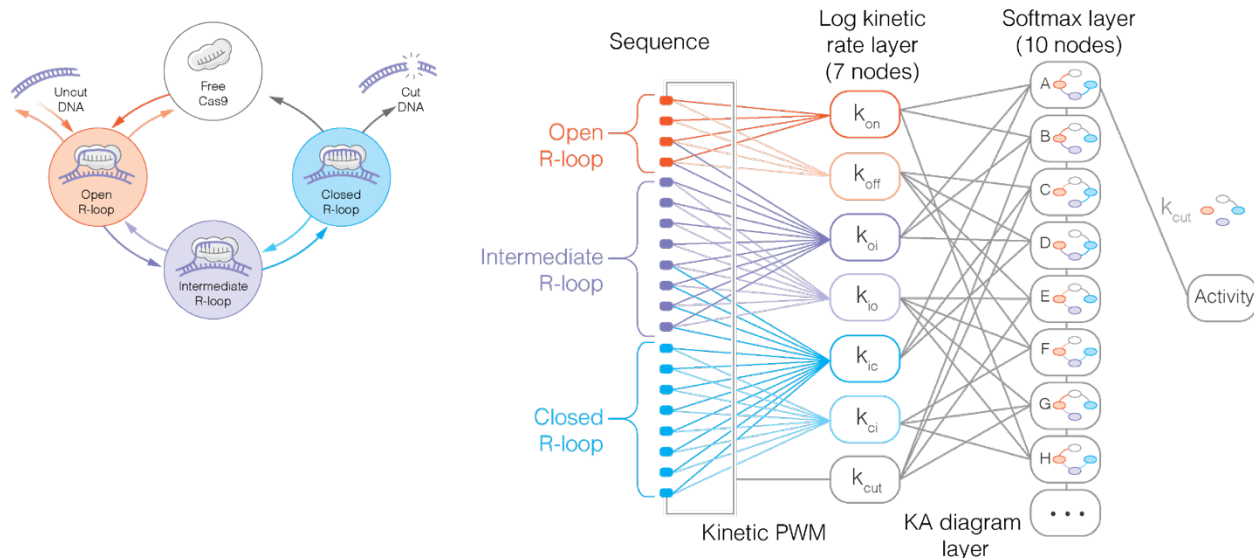

Schematic of a 4-state kinetic model of DNA cleavage by Cas9 and corresponding KINN. (Left) Diagram of kinetic model with transitions steps are color coded by arrows leading to different enzymatic states of Cas9-DNA complexes. Forward reactions are darkly colored and lead to state of the same color while reverse reactions are lighter and lead away. (Right) KINN matching the enzymatic diagram on the left. The input sequence is color coded to roughly match rates they determine. The center layer nodes' colors match the reaction step indicated in the diagram. Subscripts correspond to the starting and end state, e.g.  $k_{ic}$  is the log(kinetic rate) for reaction that goes to the Intermediates state to Closed state. A static binary layer, represented as grey lines, connects to the terms in the KA layer where subgraphs are shown to exemplify which node represents which KA diagram. A softmax is applied to this layer and the node that determines the activity, A, is multiplied by the exponentiated  $k_{cut}$  node from the Log kinetic rate layer to calculate the activity.

Extended Data Figure 11

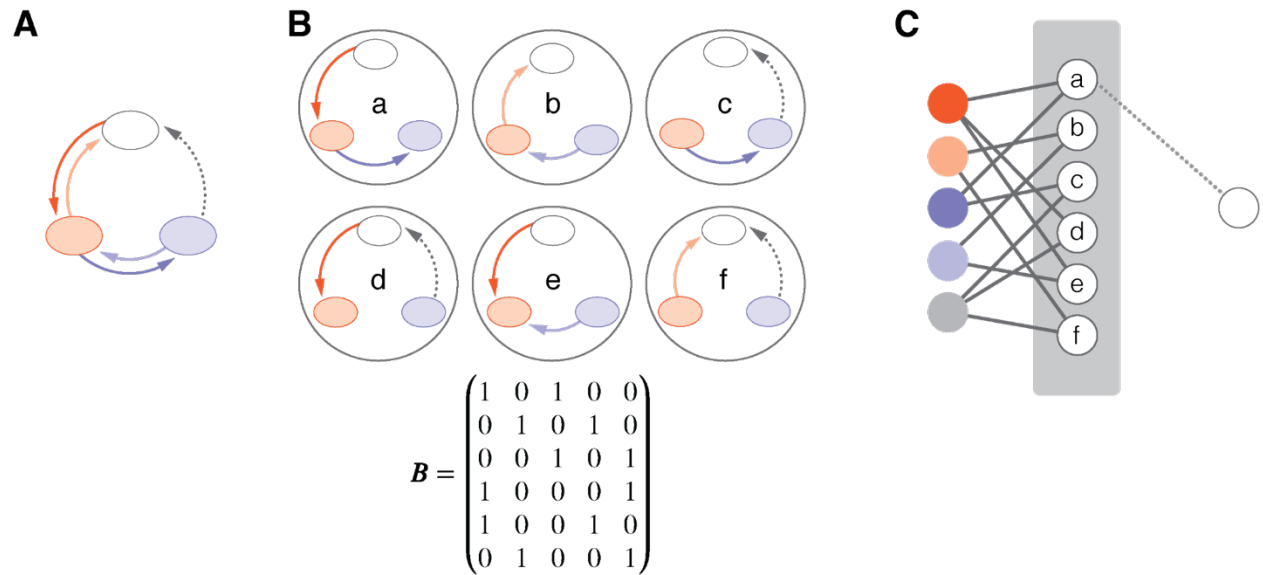

A) 3-state cas9 cleavage cycle with forward (dark red/dark purple arrows) and reverse (light red/light purple arrows) transitions for bound intermediary states (red and purple ovals). The cleavage of DNA (grey dotted arrow) is an irreversible reaction.

B) Associated King-Altman diagrams and associated binary matrix **B** for enzymatic cycle shown in A. Letters correspond to the nodes in C.

C) Full KINN architecture for reaction in A. Grey box around the second layer indicates softmax activation and dotted grey line corresponds to exponentiated value of grey node in first layer, i.e., kinetic rate constant for cleavage step.

Extended Data Table 1

Comparison of expert model\* and searched KINNs.

| Rates between enzymatic states     | Expert model | Prior sampling range | Posterior mode (gRNA 1) | Posterior mode (gRNA 2) |
|------------------------------------|--------------|----------------------|-------------------------|-------------------------|
| K <sub>ip</sub> , K <sub>pi</sub>  | [0, 12]      | [0, 22]              | [0.8, 13.5]             | [0.6, 14.7]             |
| K <sub>io</sub> , K <sub>oi</sub>  | [9, 20]      | [7, 22]              | [9.7, 20.3]             | [10.3, 20.2]            |
| K <sub>on</sub> , k <sub>off</sub> | -1           | Not searched         | -1                      | -1                      |

\*Expert model reported in Eslami-Mossallam *et al.*, 2022, *Nature Communications*.

Extended Data Table 2

|         | gRNA1             | gRNA2             |
|---------|-------------------|-------------------|
| 4-State | $0.848 \pm 0.007$ | $0.840 \pm 0.007$ |
| 5-State | $0.855 \pm 0.004$ | $0.849 \pm 0.006$ |
| 6-State | $0.861 \pm 0.002$ | $0.850 \pm 0.001$ |

Pearson correlation of predicted and observed cleavage rates using different number of states across gRNA1 and 2 datasets. Standard deviation was computed from three independent search runs.

Extended Data Table 3

| NAS runs<br>ordered by<br>validation<br>reward | TL_5                  | TL_3                  | TL_2                  | TL_1                  | TL_4                  |
|------------------------------------------------|-----------------------|-----------------------|-----------------------|-----------------------|-----------------------|
| <b>Layer 1</b>                                 | conv kernel=1         | conv kernel=1         | conv kernel=3         | conv kernel=3         | conv kernel=1         |
| <b>Layer 2</b>                                 | dropout 0.1           | dropout 0.3           | dropout 0.1           | dropout 0.3           | dropout 0.1           |
| <b>Layer 3</b>                                 | identity              | identity              | identity              | identity              | conv kernel=3         |
| <b>Layer 4</b>                                 | bidirection unit=32   | bidirection unit=32   | bidirection unit=16   | bidirection unit=32   | identity              |
| <b>Layer 5</b>                                 | flatten               | flatten               | attention flatten     | attention flatten     | attention flatten     |
| <b>Layer 6</b>                                 | dense unit=64         | dense unit=64         | dense unit=64         | dense unit=64         | dense unit=64         |
| <b>Layer 7</b>                                 | kinn 42               | kinn 62               | kinn 62               | kinn 42               | kinn 52               |
| <b>arc_tokens</b>                              | [0, 1, 5, 0, 0, 0, 1] | [0, 2, 5, 0, 0, 0, 5] | [1, 1, 5, 1, 1, 0, 5] | [1, 2, 5, 0, 1, 0, 1] | [0, 1, 1, 2, 1, 0, 3] |
